# Supplementary material for: Answering Diverse Questions via Text Attached with Key Audio-Visual Clues
Source: arXiv:2403.06679 source file (2024-03-11)
Supplement: Supplementary file 1 [file additional_tokens.tex]

\begin{figure}
\centering
\includegraphics[scale=0.6]{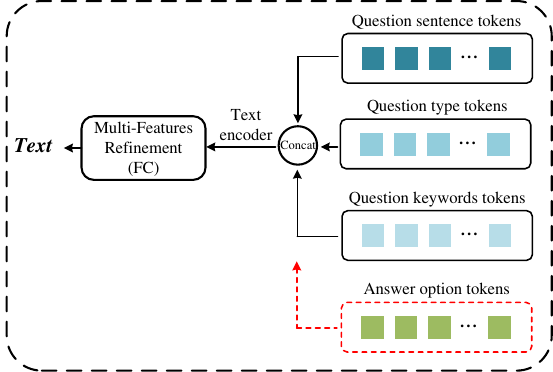}
\caption{Additional input tokens on AVQA.}
\label{fig:exp3} 
\end{figure}
